# Supplementary material for: Unified Mechanism of Atrial Fibrillation in a Simple Model
Source: arXiv:1810.12062 ancillary file (2018-10-29)
Supplement: Supplementary file 1 [file Supplementary_Material.pdf]

# Unified Mechanism of Atrial Fibrillation in a Simple Model: Supplementary Information

Max Falkenberg<sup>1,2,3</sup>, Andrew J. Ford<sup>1</sup>, Anthony C. Li<sup>1</sup>, Alberto Ciacchi<sup>1,2,3</sup>, Nicholas S. Peters<sup>3</sup>, Kim Christensen<sup>1,2,3\*</sup>

<sup>1</sup>Blackett Laboratory, Imperial College London, London SW7 2AZ, United Kingdom

<sup>2</sup>Centre for Complexity Science, Imperial College London, London SW7 2AZ, United Kingdom

<sup>3</sup>ElectroCardioMaths Programme, Imperial Centre for Cardiac Engineering, Imperial College London, London W12 0NN, United Kingdom

(Dated: October 29, 2018)

## I. MODEL DEFINITION

**Heart muscle structure.** The area of the atrial muscle is  $L'_x \times L'_y \approx 20\text{cm}^2$  [1, 2] while the thickness of the atrial muscle wall ranges from 1mm to 7mm [3]. A typical average is about  $L'_z = 2.5\text{mm}$  [4]. The atrial muscle tissue comprises tubular shaped heart muscle cells (myocytes) of length  $\Delta x' \approx 100\mu\text{m}$  and diameter  $\Delta y' = \Delta z' \approx 20\mu\text{m}$  [5, 6]. Cells are predominantly connected longitudinally, forming fibres that connect transversally now and again. Hence a branching network of anisotropic cells provides an appropriate picture of the atrial tissue.

**Heart muscle physiology.** The membrane potential of heart muscle cells shows that they can be in one of three states: excited, where the cell depolarises, resting, where the cell can be depolarised by a neighbouring active cell, and refractory, where for some time  $\tau'$  after excitation the cell cannot be re-excited. The shortest time scale is associated with a cell depolarising,  $\Delta t' \approx 0.6\text{ms}$ , whereas the refractory period lasts  $\tau' \approx 150\text{ms}$ . When a resting cell is induced to excite by a neighbouring excited cell, it contracts. The propagation speed of the activation wavefront is  $\Delta x'/\Delta t' \approx 0.2\text{ms}^{-1}$  and the heart's natural pacemaker (sinus node) ensures the periodic propagation of a coordinated activation wavefront, causing atrial muscle contractions. The rate of excitations are controlled by the pacemaker cells that regularly self-excite with period  $T' = 300 - 1000\text{ms}$ . For example  $T' = 660\text{ms}$  corresponds to approximately 90 beats per minute.

**Dimensionless parameters of the model.** We can translate real tissue values into dimensionless model parameters. We apply a similar conversion procedure to that presented in Ref. [7]. The dimension of the simplified 3d topology are  $L_x = L'_x/\Delta x' = 1000$ ,  $L_y = L'_y/\Delta x' = 1000$  and  $L_z = L'_z/\Delta z' = 125$ . We apply a coarse grain transformation  $\Delta x' \rightarrow b\Delta x'$ ,  $\Delta y' \rightarrow b\Delta y'$ ,  $\Delta z' \rightarrow b\Delta z'$  such that we group  $b^3$  cells within one node of the model. The propagation speed has to remain constant  $\Delta x'/\Delta t' \approx 0.2\text{ms}^{-1}$  so we must also coarse grain time  $\Delta t' \rightarrow b\Delta t'$  [7]. By using  $b = 5$ , we find the dimensionless parameters of the model. For the 3d pipe structure, we have  $L_x = L'_x/(b\Delta x') = 200$ ,  $L_y = L'_y/(b\Delta y') = 200$  and  $L_z = L'_z/(b\Delta z') = 25$ . The renormalised excitation

time  $b\Delta t' = 3\text{ms}$  yields a dimensionless refractory period  $\tau = \tau'/(b\Delta t') = 50$  and pacemaker activation period  $T = T'/(b\Delta t') = 220$ , assuming  $T' = 660\text{ms}$ .

**Modelling the real atrial tissue.** The structural properties presented above are mimicked by a simple 3d pipe-like topology of the atria,  $L_x \times L_y \times L_z$ , where  $x$  is the longitudinal direction and  $y$  and  $z$  the transverse directions. The pacemakers cells are identified with the nodes at the boundary  $x = 0$ . Hence, we apply open boundaries in  $x$  and  $z$  and periodic boundaries in  $y$ . Each of the  $L_z = 25$  layers contain  $L_x \times L_y = 200 \times 200$  nodes. The nodes are connected longitudinally with frequency  $\nu_{\parallel}$  and transversally (within the layer and across layers) with frequency  $\nu_{\perp}$ . The network of nodes mimic the branching structure of heart muscle fibres.

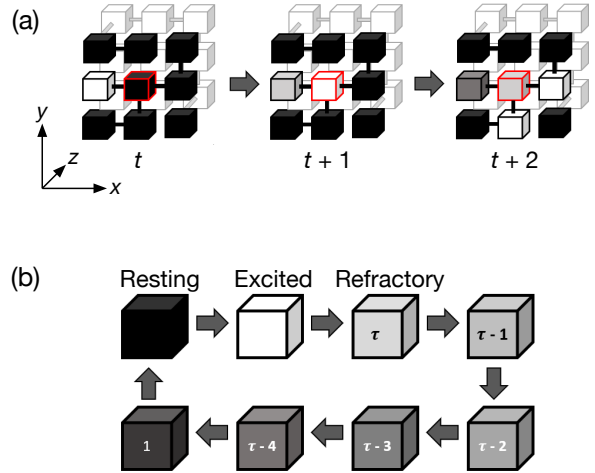

FIG. 1. (a) The excitation wave propagates across neighbouring nodes. Nodes are connected longitudinally with frequency  $\nu_{\parallel}$  and transversally (along  $y$  and  $z$  directions) with frequency  $\nu_{\perp}$ . At time  $t$ , the red bordered node is resting. At time  $t+1$ , the node activates in response to the stimulus coming from its neighbour to the left. At time  $t+2$ , the red bordered node becomes refractory and the excitation wave activates the two nodes in resting state to which it is coupled. The node to the left of the red bordered node cannot be excited as it is in a refractory state. (b) Temporal dynamics of a node. Each node sequentially passes across three distinct states: resting (black), excited (white) and refractory (grey scale).

\* Corresponding Author: k.christensen@imperial.ac.uk

To mimic the membrane potential of a cell, nodes can be in one of three distinct states: resting, excited or

refractory. At a given time  $t$ , an excited cell induces resting cells to which it is coupled to excite at time  $t + 1$ . The excited cell at time  $t$  becomes refractory at time  $t + 1$  and it will not be able to respond to any further stimulus during the next  $\tau$  time steps. The refractory cell will revert to a resting cell after  $\tau$  time steps, see Fig. 1.

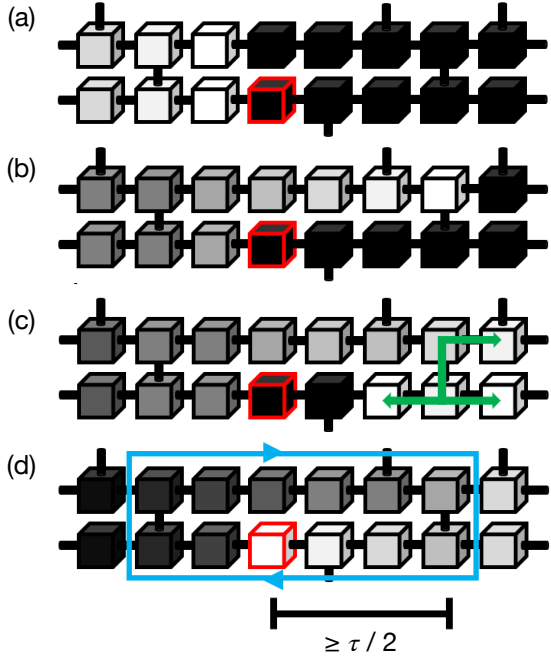

FIG. 2. Progression of the excitation wave through a simple re-entrant circuit situated on the surface of the 3d topology used to mimics the muscle fibre network. The red bordered cell may act as a conduction block. (a)-(b) The planar excitation wave reaches the node that is susceptible to conduction block. The red bordered node did not excite and blocked the propagation in the lower fibre while the planar propagation of the wavefront proceeds in the upper fibre. (b)-(c) The activation wavefront reaches the penultimate node in the upper fibre that connects the two adjacent fibres. The excitation advances in multiple directions, indicated with the green arrows. In particular, the wavefront leaks back in the fibre where the original conduction was blocked. (c)-(d) If the path length indicated in the lower fibre is longer than  $\tau/2$ , the node placed to the left of the red bordered node will have reached its resting state when the backward propagation arrives. Therefore, the region indicated in light blue will act as a re-entrant circuit until the red bordered node blocks the excitation again. The likelihood of creating a re-entrant circuit is determined by the coupling frequencies  $\nu_{\parallel}$  and  $\nu_{\perp}$  and  $\delta$ . Large values of  $\nu_{\parallel}$  yield long, uninterrupted longitudinal fibres. Large values of  $\nu_{\perp}$  implies a well connected network with no re-entrant circuits possible. Decreasing  $\nu_{\perp}$  allows re-entrant circuits to emerge.

A small fraction  $\delta$  of the nodes can be susceptible to conduction block. These nodes are selected at random and their position in the network is fixed for a given realisation. These particular nodes will, with a small probability  $\epsilon$ , fail to activate when their neighbours excite. In a well connected network, such a failure will not

disrupt the planar propagation of the excitation wave and sinus rhythm prevails. However, if the network of heart muscle cells becomes too decoupled, for example due to fibrosis, then, when a failure occurs, the planar propagation of the excitation wave may be disrupted. The break of the regular wave front may prompt the spontaneous emergence of circuits formed by wavelets of excitation leaking back through the refractory wake of the wave front [7]. However, this only occurs if nodes in a certain region of the atrial muscle form a particular configuration called a re-entrant circuit, see Fig. 2. Re-entrant circuits can emerge spontaneously in the atria due to structural changes during the lifetime of a patient as specific pathologies (e.g., fibrosis) might decrease the coupling between cells.

The critical structures discussed in Fig. 2 have been introduced by Christensen, Manani and Peters in [7]. In the three-dimensional network, similar configurations are relevant but now they can be placed within the bulk as well as on the endo- and epicardial surfaces. Indeed, the behaviour of the model predicts that local re-entrant drivers of persistent AF are located in the bulk of the atrial muscle rather than on the surface, see Fig. 3.

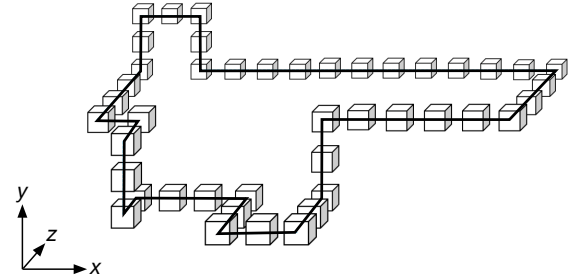

FIG. 3. Three-dimensional visualisation of an AF driver located in the bulk of the atrial tissue. The black path represents the connectivity structure between the nodes. In this particular example we observe that longitudinal connections are more frequent than transverse connections ( $y$  and  $z$  directions), representative of re-entrant circuits that can be observed when  $\nu_{\parallel}$  is substantially larger than  $\nu_{\perp}$ .

## II. DATA VISUALISATION

The raw model data contains small scale noise which obscures the overall behaviour. Therefore, to effectively visualise model activity, the raw data needs to be filtered in a manner mimicking real clinical imaging techniques. The optical mapping system used by Ref. [3] recorded to a depth of 1 – 4 mm weighted to the layer being observed, with a resolution of approximately 0.02 mm. This data guided the coarse graining: The activation patterns were convolved with a 3d Gaussian, with standard deviations  $\sigma_x = \sigma_y = 1$  and  $\sigma_z = 5$ . The differences between the

raw and processed images are shown in Fig. 4.

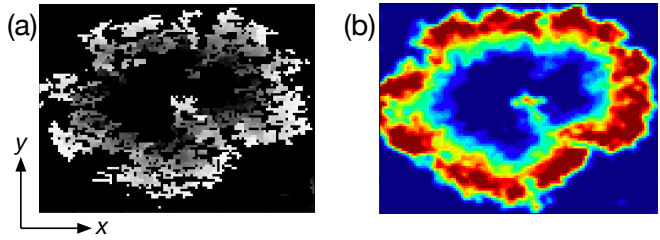

FIG. 4. Surface activation patterns in the model (a) before and (b) after processing. (a) The raw cell states of a single layer of nodes in the model. White indicates active cells, black nodes are resting (excitable), and grey cells are refractory. This raw image only shows the cell states in a single layer at a fixed  $z$  coordinate. (b) To aid data interpretation and match the visualisation methods applied in Ref. [3] we process the raw image using Gaussian smoothing. A 3d Gaussian kernel is used to convolve the raw cell states. The Gaussian is centred on the imaged surface with standard deviations  $\sigma_x = \sigma_y = 1$  and  $\sigma_z = 5$ . The colour scheme for the activation maps after processing has been chosen to match that used in Ref. [3]. Active wavefronts are shown in red, resting nodes are in blue, and refractory nodes are represented by all other colours. This filtered image improves the coherence of wavefronts in the model and aids data interpretation. Scale:  $100 \times 75$  nodes.

### III. FURTHER MODEL RESULTS

**Activation Maps.** In the model, we observe a wide variety of surface activation maps. These can be characterised as full surface re-entry (where the active wavefront is visible for the full re-entry cycle), partial surface re-entry (where only part of the re-entry cycle is visible), single location breakthrough points, and multiple quasi-simultaneous breakthrough points. The surface activity that is observed in any given tissue depends on the depth of the re-entrant circuit as well as the level of connectivity in the tissue. Close-up breakthrough point activation maps are shown in Fig. 5, full and partial re-entry maps are shown in Fig. 6.

For a re-entrant circuit located in the bulk, both the endocardial and epicardial activation maps are similar, as shown in Fig. 7. A stronger delay can be seen for circuits on one surface. Re-entrant circuits are seen on the endocardium and epicardium in Fig. 8 and Fig. 9 respectively. Breakthrough points are observed on the surface opposite the re-entrant circuit.

A cross-section of the model at fixed  $y$  coordinate is shown in Fig. 10, where the top (bottom) of each image corresponds to the epicardium (endocardium). The cross-section is aligned with a re-entrant circuit near the endocardium. The figure shows how the activation continuously propagates around the re-entrant circuit in a spiral manner. Fibrillatory waves are emitted from the end of the isolated fibre and spread through the bulk towards the

epicardium. The anisotropic fibre structure in the atrial wall results in an uneven wavefront and, consequently, complex breakthrough patterns on the epicardial surface.

**Depth of re-entrant circuits.** We can measure the depth from the endocardium ( $z$  coordinate) at which re-entrant circuits form in the homogeneous and inhomogeneous model. Figure 11 (Fig. 12) shows the distribution of re-entrant circuit depths for the homogeneous (inhomogeneous) model at various points on the model's risk curve, shown in Fig. 2a (Fig. 2b) in the main manuscript.

In the homogeneous model, the fibre structure is statistically equivalent across the whole tissue. Hence, there is no distinction between the endocardial surface at  $z = 0$  and the epicardial surface at  $z = 24$ . Figure 11 shows that in paroxysmal AF, re-entrant circuits form preferentially near the atrial surfaces. As cells continue to decouple and the model approaches persistent AF, re-entrant circuits form uniformly in the bulk. This dependence of re-entrant circuit depth on AF persistence is found to exist for models with strong longitudinal and weak transverse coupling (Fig. 11 left column), equal longitudinal and transverse coupling (Fig. 11 central column), and weak longitudinal and transverse coupling (Fig. 11 right column). However, re-entrant circuits cluster around the atrial surfaces more closely for strong longitudinal with weak transverse coupling, than for weak longitudinal and strong transverse coupling.

As a result, when the fibre orientation is varied in the inhomogeneous model, re-entrant circuits will form preferentially in the regions with the strongest longitudinal coupling. This breaks the symmetry in re-entrant circuit distribution between the endocardium and the epicardium in the inhomogeneous model. In the inhomogeneous model for paroxysmal AF, re-entrant circuits are found to cluster preferentially at the atrial surfaces, as opposed to uniformly in the bulk, and at the endocardium, as opposed to the epicardium. As AF progresses, the asymmetry between epicardium and endocardium weakens and re-entrant circuits move deeper into the bulk of the atrial wall. Hence, the average distance of re-entrant circuits from the endocardial surface increases as AF becomes more persistent. As re-entrant circuits move deeper into the atrial wall, they become harder to ablate.

**Ablation in the Model.** We can simulate ablation in the model by permanently disabling a set of nodes corresponding to the desired ablation lesion. In clinical practice, ablation is carried out by burning lesions from the endocardial surface.

By ablating active re-entrant circuits in the model, AF can be terminated and the model will return to sinus rhythm. An example of this process is shown in Fig. 13. By ablating part of the re-entrant circuit, the back propagating excitation is blocked from re-entering the excitable tissue and the fibrillatory activity dissipates.

In clinical practice, ablation lesions can typically only penetrate up to 2mm into the atrial wall from the endocardial surface. The atria is 1-7mm thick [3], averaging approximately 2.5mm [4]. As a result, re-entrant circuits

which are far from the endocardium may be difficult to destroy using ablation.

Figure 14 demonstrates the effect of variable ablation depth in the model. In the figure, there are two active re-entrant circuits, one near the endocardium and one near the epicardium. Applying shallow ablation lesions to the surface at the position of both re-entrant circuits, the circuit near the endocardium is destroyed. However, the circuit near the epicardium remains active. Hence, ablation has failed and the model remains in AF. Repeating this process with ablation lesions which penetrate the full distance through the atrial wall, both re-entrant circuits are destroyed and fibrillatory activity dissipates. As a result, the model returns to sinus rhythm. Note however that ablating active re-entrant circuits does not prevent new re-entrant circuits forming in other regions of the tissue with significant cell-to-cell decoupling. Additionally, new re-entrant circuits may form if nodes continue to decouple. In persistent AF, the number of possible re-entrant circuits is so great that it is often not possible to successfully return the tissue to sinus rhythm if these circuits are destroyed.

#### IV. VIDEOS

Videos of the activation patterns observed in the model can be found in the supplementary material. Captions for the videos are listed below. All videos are for the inhomogeneous model where the average cell-to-cell coupling is fixed,  $\bar{\nu} = \text{constant}$ , and variation in fibre direction varies linearly from  $\Delta\theta_{\text{ENDO}} = 24^\circ$  at the endocardium ( $z = 0$ ) to  $\Delta\theta_{\text{EPI}} = 42^\circ$  at the epicardium ( $z = 24$ ). The model has dimensions  $L_x = L_y = 200$  and  $L_z = 25$  as outlined in the model definition in section I. The remaining model parameters are  $\delta = 0.05$ ,  $\epsilon = 0.05$ ,  $\tau = 50$  and  $T = 220$ .

**Videos A.** Close-up videos of the endocardium and the epicardium showing the spontaneous emergence of AF in the inhomogeneous model,  $\bar{\nu} = 0.31$ . A re-entrant circuit forms near the endocardial surface. This video corresponds to Fig. 1 and Fig. 3c in the main manuscript. The epicardial breakthrough is shown in Fig. 5(a) in the supplementary material.

**Videos B.** Close-up videos of the endocardium and the epicardium showing the spontaneous emergence of AF in the inhomogeneous model,  $\bar{\nu} = 0.33$ . A re-entrant circuit forms near the endocardial surface. This video corresponds to Fig. 8 in the supplementary material. The epicardial breakthrough is shown in Fig. 5(b) in the supplementary material.

**Videos C.** Close-up videos of the endocardium and the epicardium showing the spontaneous emergence of AF in the inhomogeneous model,  $\bar{\nu} = 0.32$ . A re-entrant circuit forms near the endocardial surface. The epicardial breakthrough is shown in Fig. 5(c) in the supplementary material.

**Videos D.** Close-up videos of the endocardium and the epicardium showing the spontaneous emergence of

AF in the inhomogeneous model,  $\bar{\nu} = 0.31$ , and a cross section through the atrial wall showing the formation of a re-entrant circuit near the endocardial surface and the propagation of fibrillatory waves through the atrial wall to the epicardium. The endocardial view in this video corresponds to Fig. 6(b) in the supplementary material. The cross section corresponds to Fig. 10 in the supplementary material.

**Videos E.** Close-up videos of the endocardium and the epicardium showing the spontaneous emergence of AF in the inhomogeneous model,  $\bar{\nu} = 0.32$ . A re-entrant circuit forms near the endocardial surface. The epicardial breakthrough is shown in Fig. 5(e) in the supplementary material.

**Video F.** A full scale video showing the simultaneous activation patterns on the endocardium and epicardium, and cross sections through the atrial wall,  $\bar{\nu} = 0.32$ . The video shows many of the key features of emergent AF in the model. The model starts in sinus rhythm before a single re-entrant circuit forms. This circuit forms temporarily and dies out after one cycle. This temporary circuit forms three times before a new sustained re-entrant circuit emerges near the endocardium. The new sustained circuit drives fibrillatory activity across the tissue blocking new wavefronts from entering the tissue at the pacemaker,  $x = 0$ . Shortly after time 2000, the re-entrant circuit is ablated and fibrillatory waves dissipate. However, the interaction between the dissipating fibrillatory waves and a new pacemaker wavefront results in a new short lived circuit forming at time 2500. The new fibrillatory waves dissipate before the tissue returns to sinus rhythm. Note that the ablation lesion disrupts all future sinus rhythm wavefronts, although the effect is small.

**Video G.** A full scale video showing the emergence of AF before being terminated by ablation,  $\bar{\nu} = 0.33$ . The re-entrant circuit forms near the endocardium before being destroyed by ablation. The fibrillatory waves dissipate before the tissue returns to sinus rhythm.

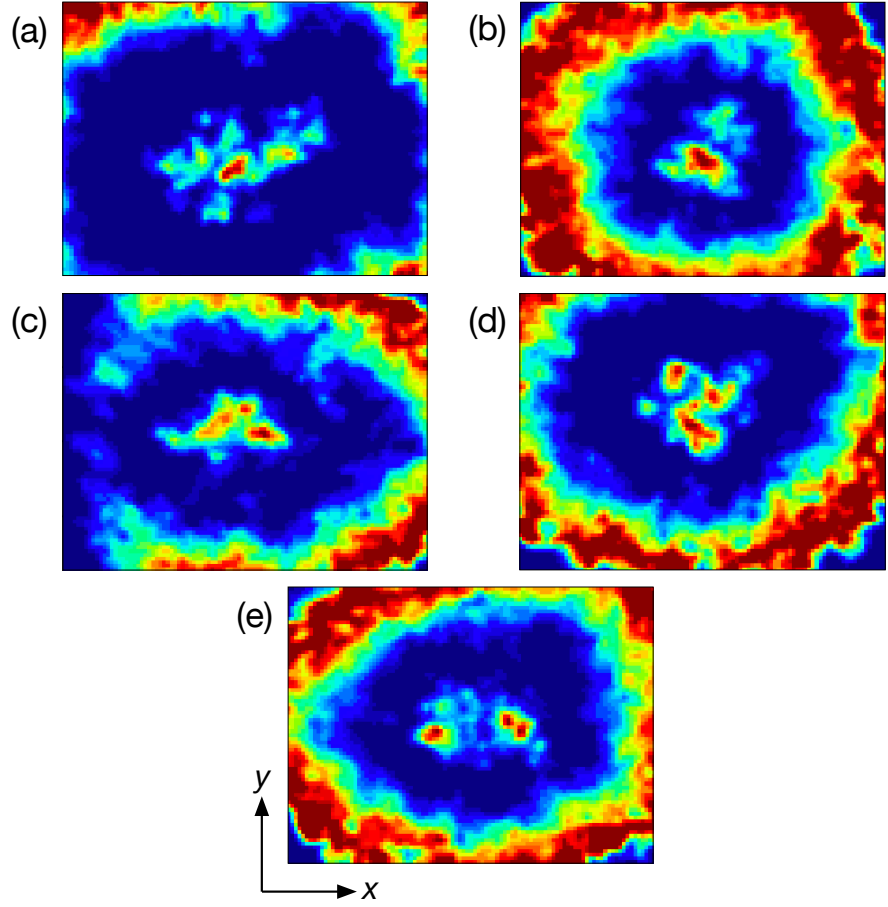

FIG. 5. Examples of breakthrough patterns in the model. Close-up view of activity for five different realisations (tissues). Tissues (a) and (b) show one primary breakthrough point. Tissues (c) and (d) show the activity emerging across a wider area almost simultaneously. Tissue (e) shows two clearly divided breakthrough points. Globally, all five tissues have breakthrough activity that will generate waves that appears to originate from a focal point. These activation patterns are typical observed on the epicardium during paroxysmal AF, but may in rare cases also be seen on the endocardium. Quantitatively differentiating between breakthrough types is difficult. See videos A–E. Scale:  $100 \times 75$  nodes.

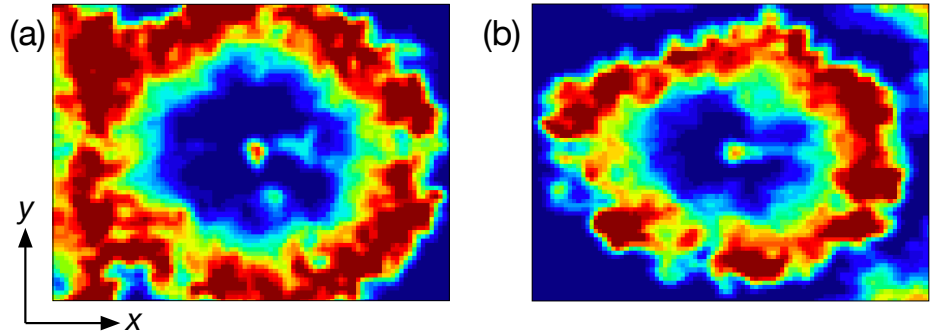

FIG. 6. Examples of partial and full re-entry in the model. (a) An example of partial surface re-entry where a full rotation is not observed in the surface activity. This is because the re-entrant stretches to a depth of approximately 4 nodes from the endocardial surface. (b) Complete surface re-entry, where no gaps are observed in the re-entrant circuit. Re-entrant circuits are typically observed on the endocardium during paroxysmal AF, but may also be found on the epicardium in rare cases. Scale:  $90 \times 70$  nodes.

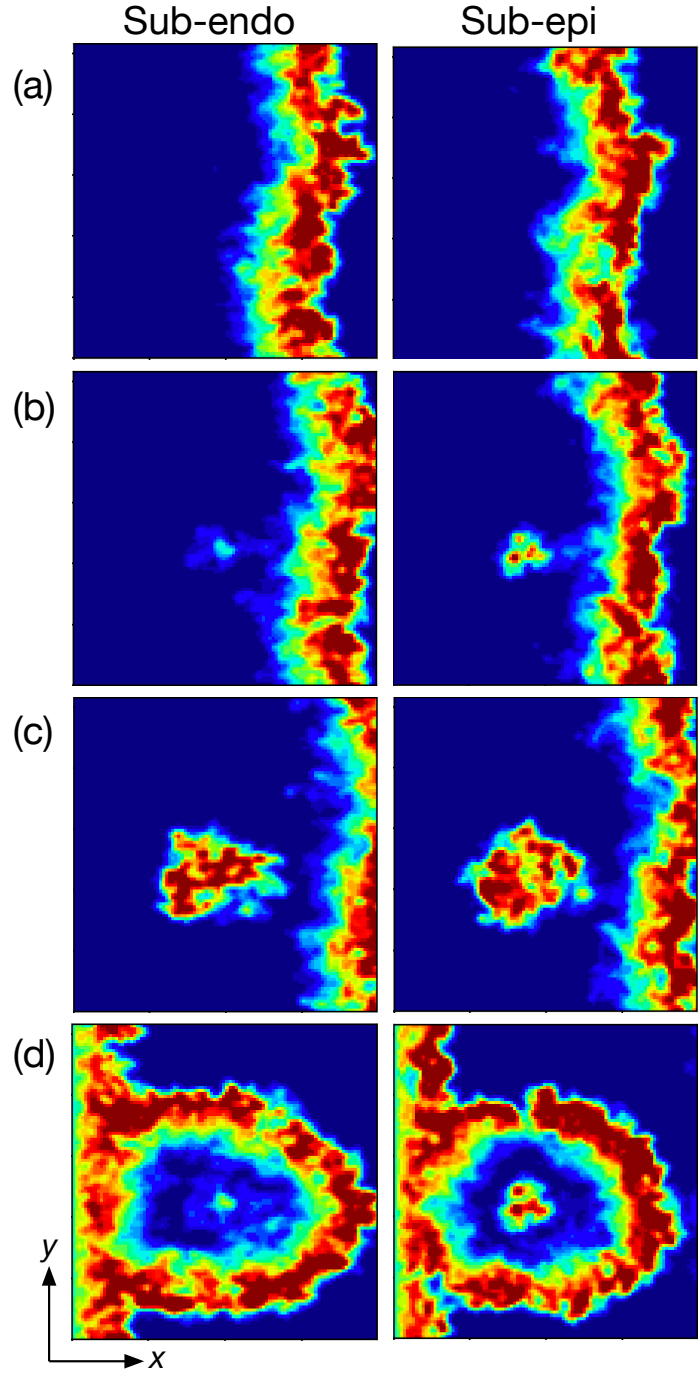

FIG. 7. An example of surface activation patterns where re-entrant activity is not observed on either atrial surface. Close-up view of activation pattern in the case of a re-entrant circuit with depth  $z = 16$ ,  $\bar{\nu} = 0.31$ . (a) The tissue in sinus rhythm with regularly propagating wavefronts. A signature of fibrillatory activity characterising AF is not observed. (b) Initial fibrillatory activity emerges on both epicardium and endocardium as breakthrough points. Note that this re-entrant circuit is 8 layers closer to the epicardium than the endocardium, as can be seen by the delay between activation patterns. (c) Fibrillatory activity spreads across the tissue. (d) AF is sustained. Re-entrant circuits are not observed on either surface. Scale:  $100 \times 100$  nodes.

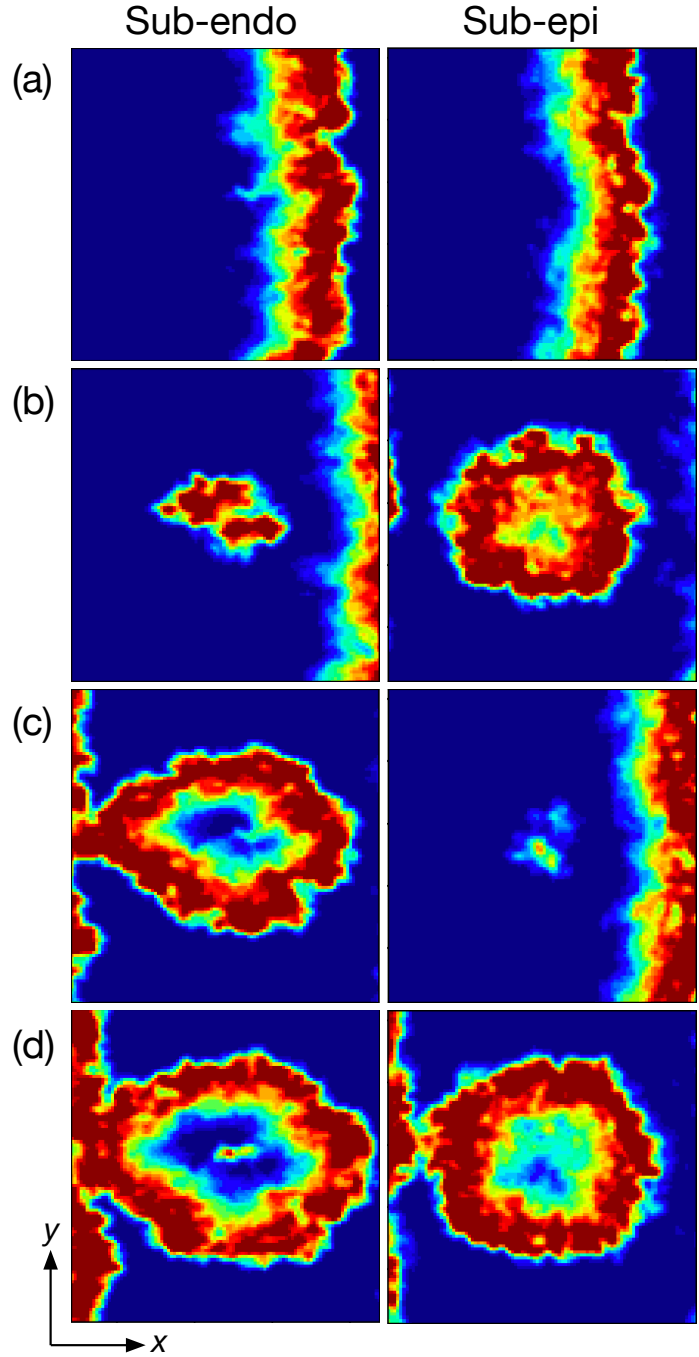

FIG. 8. An example of re-entrant activity observed on the endocardial surface. Close-up view of activation patterns in the case of a re-entrant circuit near the endocardial surface with depth  $z = 1$ ,  $\bar{\nu} = 0.33$ . (a) The model in sinus rhythm. A faint re-entrant excitation is observed at the centre of the sub-endo view. (b) Fibrillatory activity emerges in the model. An unexcited tract on the right side of the active region in the sub-endo view indicates the isolated fibre for the re-entrant circuit. Activity spreads on the sub-epi view resembling a focal source. (c) The wavefront re-enters the unexcited tract in the sub-endo view. The activity breaks through onto the epicardial surface at a single stable breakthrough point. (d) Fibrillatory activity is sustained. Scale:  $100 \times 100$  nodes.

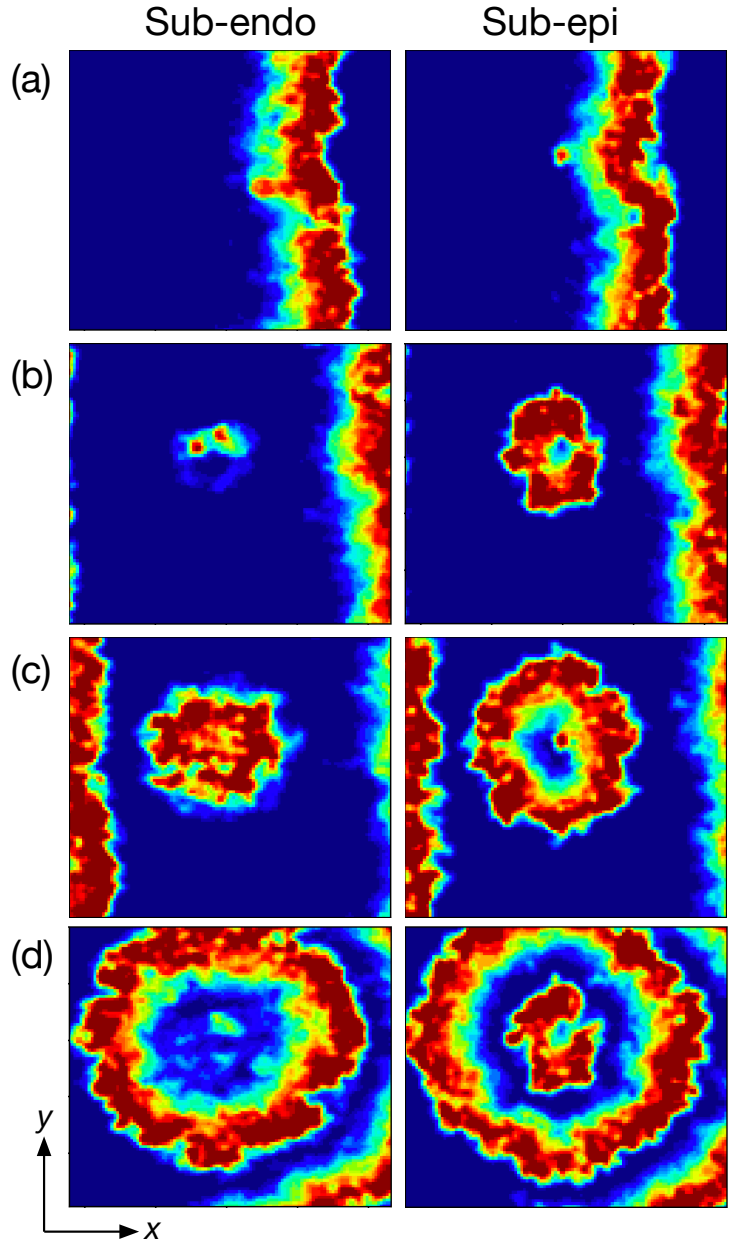

FIG. 9. An example of re-entrant activity observed on the epicardial surface. Close-up view of activation pattern in the case of a re-entry circuit near the epicardium with depth  $z = 22$ ,  $\bar{\nu} = 0.32$ . Circuits forming near the epicardium are much rarer than those forming near the endocardium in paroxysmal AF. (a) The model in sinus rhythm. A faint re-entrant excitation is observed above the centre of the sub-epi view. (b) Fibrillatory activity emerges in the model. An excitation is just starting to enter the unexcited tract on the right side of the active region in the sub-epi. Fibrillatory activity has broken through to the endocardial surface at multiple points simultaneously. (c) & (d) Fibrillatory activity is driven and sustained. A re-entrant circuit is clearly observed from sub-epi imaging. Activity appears to originate from a focal point in sub-endo imaging. Scale:  $110 \times 100$  nodes.

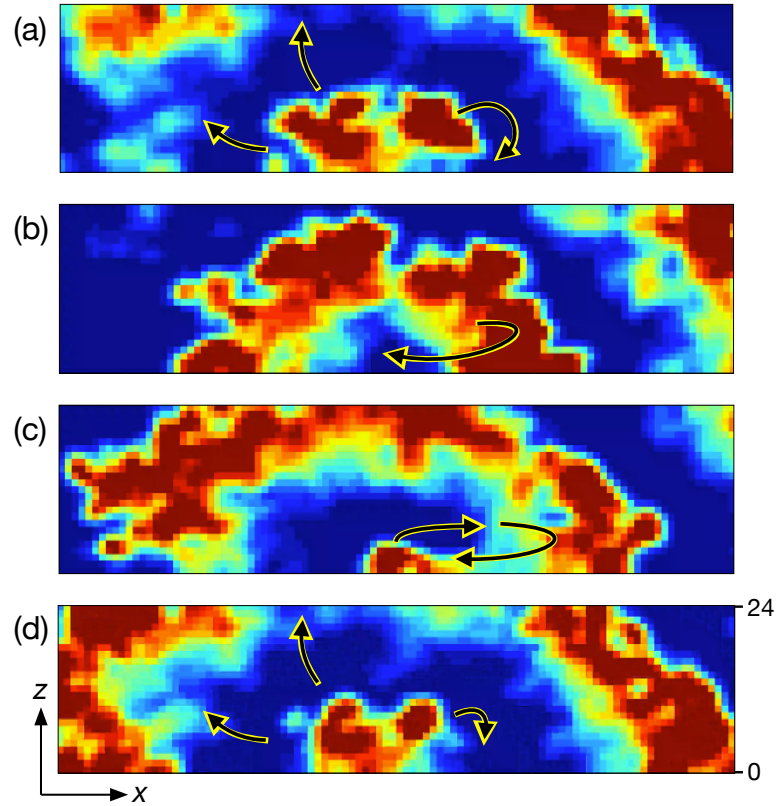

FIG. 10. A cross-section of the model during AF showing a close-up of the  $x$ - $z$  plane (fixed  $y$  coordinate). The cross-section has been chosen to align with a re-entrant circuit. Arrows indicate the movement of wavefronts. The top (bottom) surface of each panel corresponds to the epicardium (endocardium). A re-entrant circuit can be seen near the endocardium with (a) activity moving around an isolated fibre, (b) & (c) re-entering the isolated fibre, and (d) emitting fibrillatory waves from the left end of the isolated fibre. Fibrillatory activity spreads from the endocardium to the epicardium through the complex fibre structure of the model. This results in a wide variety of possible breakthrough patterns on the epicardial surface. When viewed from the endocardium, re-entrant activity will be clearly visible since the isolated fibre lies along the endocardial surface. When viewed from the epicardial surface, the wavefronts propagating from the re-entrant circuit may emerge as a single breakthrough point, or as multiple breakthrough points simultaneously. See video D. Scale:  $100 \times 25$  nodes.

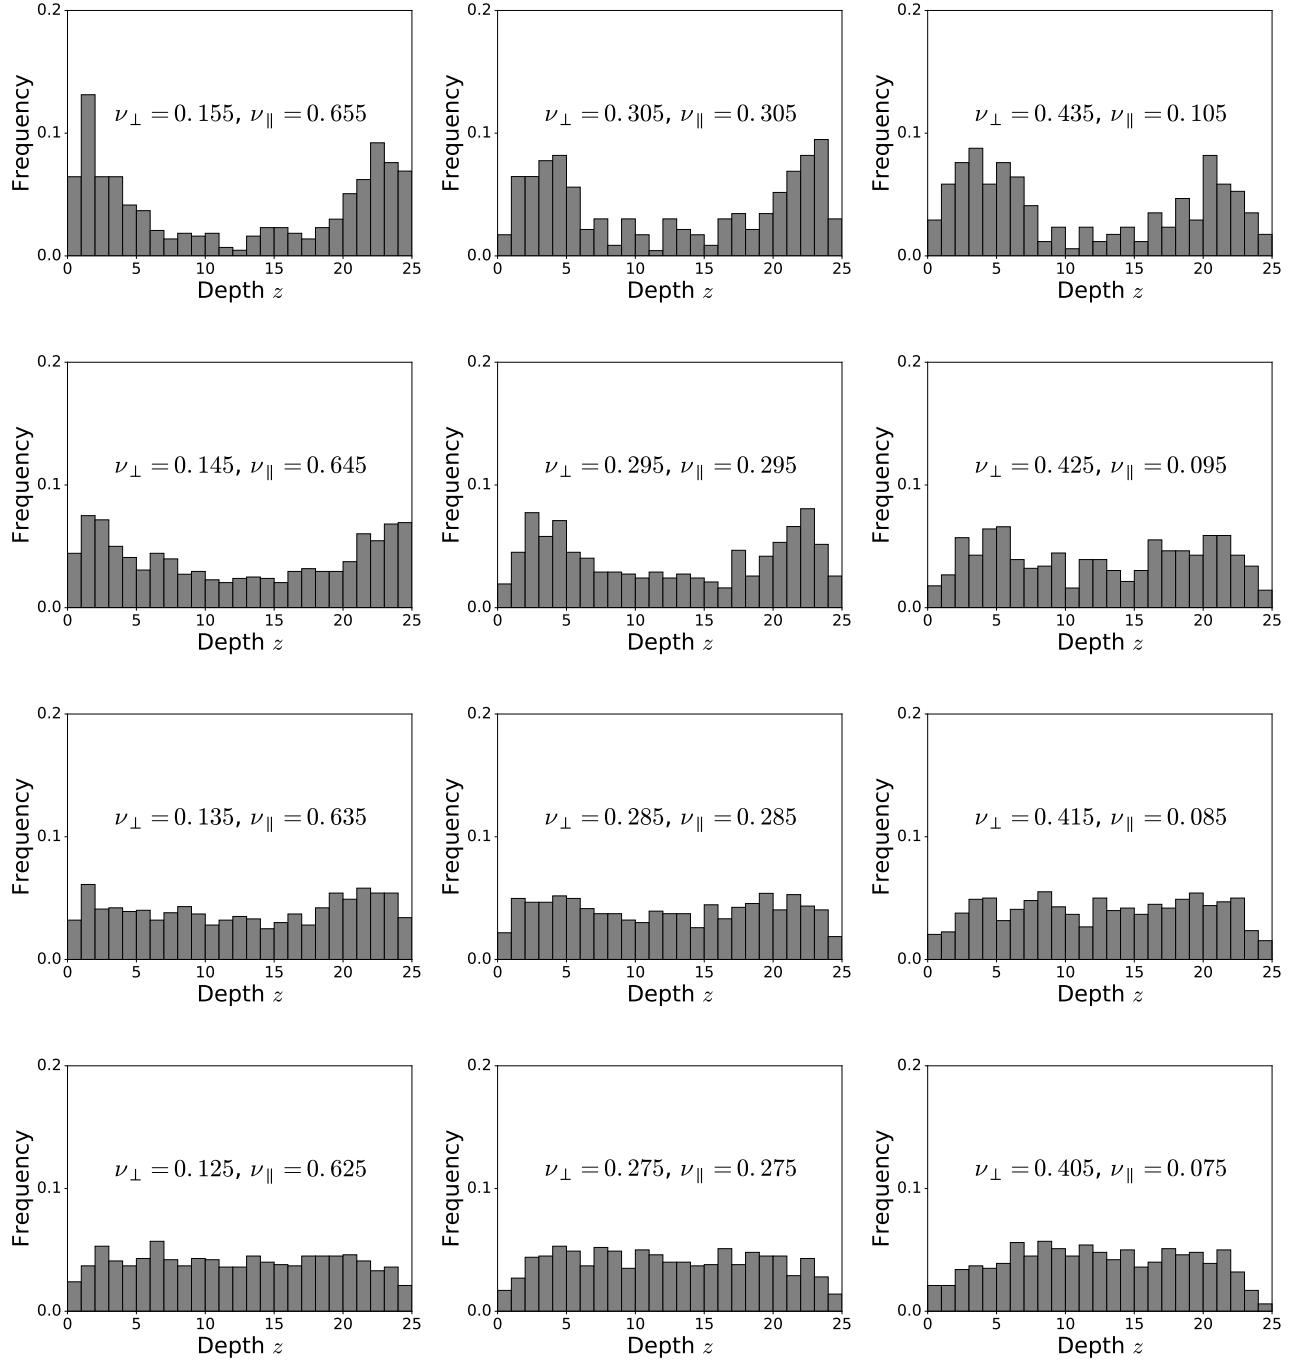

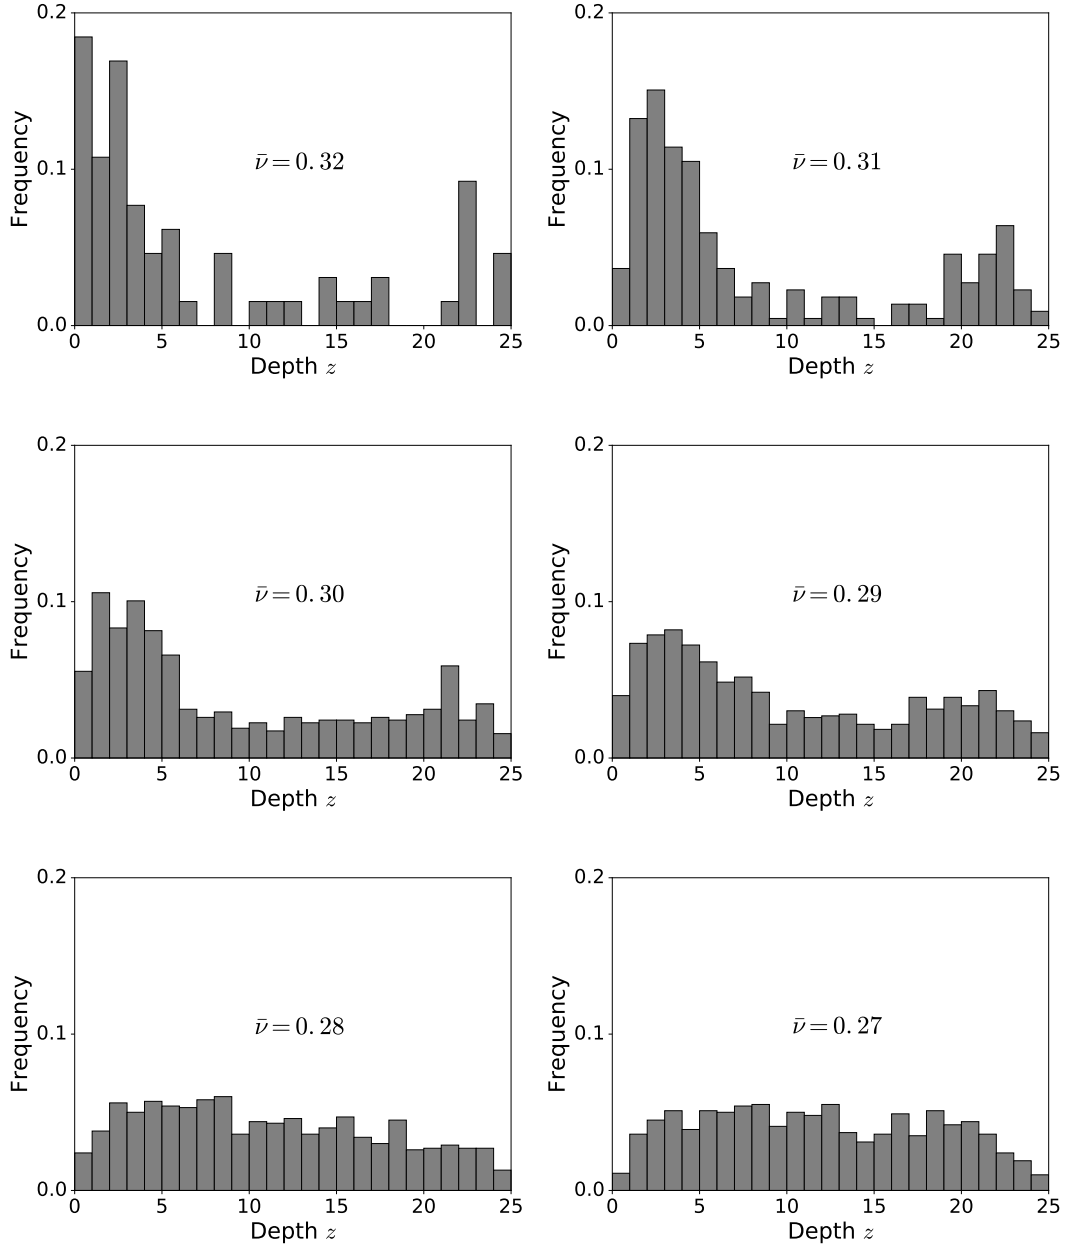

FIG. 12. The distribution of re-entrant circuit depth  $z$  from the endocardium in the inhomogeneous model. AF progresses from paroxysmal AF ( $\bar{\nu} = 0.32$ ) to persistent AF ( $\bar{\nu} = 0.27$ ). Fibre angle varies linearly across the tissue from  $\Delta\theta_{\text{ENDO}} = 24^\circ$  on the endocardium to  $\Delta\theta_{\text{EPI}} = 42^\circ$  on the epicardium. Depth  $z = 0$  ( $z = 24$ ) corresponds to the endocardium (epicardium). In the inhomogeneous model, the symmetry between the epicardium and endocardium is broken with the stronger longitudinal coupling on the endocardium than the epicardium. For paroxysmal AF, re-entrant circuits are predominantly found near the atrial surfaces, and significantly more circuits cluster near the endocardium than the epicardium. This is because fibres have much stronger longitudinal coupling on the endocardial surface than on the epicardial surface. When visualised from the endocardium, these circuits will typically appear as re-entrant or rotational activity. In persistent AF, re-entrant circuits are uniformly distributed in the bulk of the atrial wall, away from the epicardium and endocardium. These circuits are more likely to result in focal or breakthrough activation patterns when visualised from the endocardium. As AF has progressed from paroxysmal to persistent, the average depth of circuits from the endocardium at  $z = 0$  has significantly increased – this hinders the effective use of catheter ablation for those circuits deep in the atrial bulk.

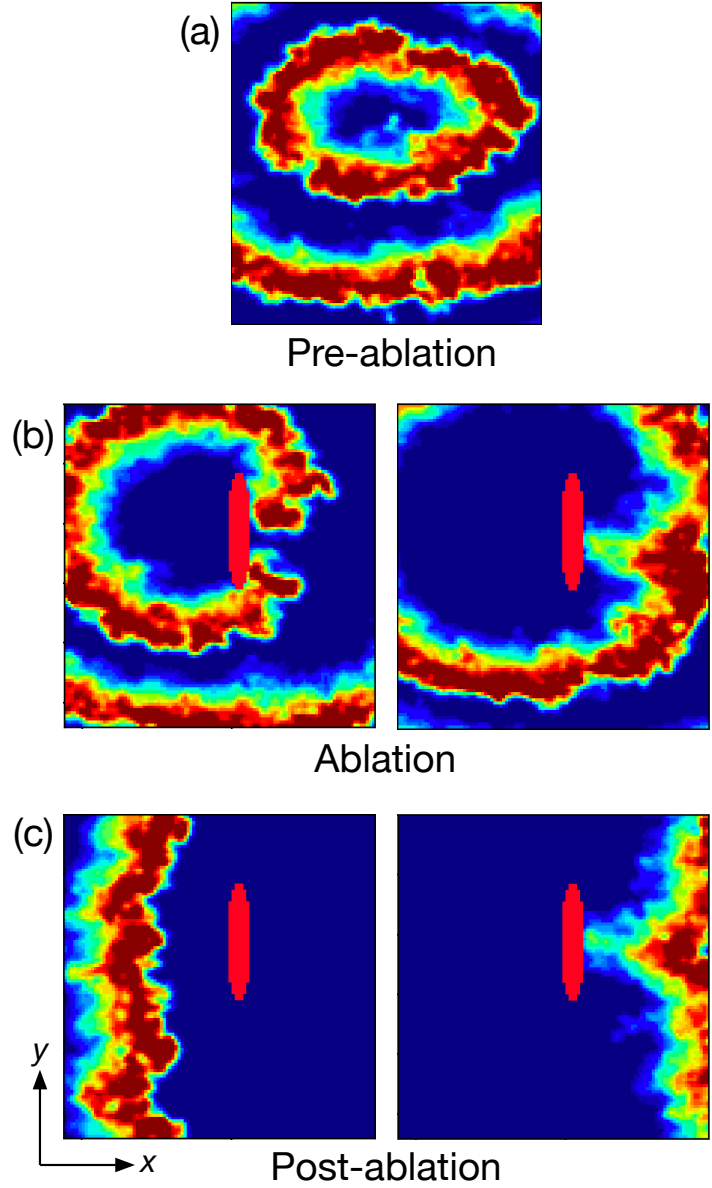

FIG. 13. The termination of AF by destroying the re-entrant circuit using ablation in the inhomogeneous model. The images show the activation patterns for a close-up of the endocardial surface. (a) A faint re-entrant excitation is visible just above the centre of the image. This corresponds to the re-entrant circuit which is driving AF. (b) Nodes surrounding the re-entrant circuit are destroyed (solid red region). The re-entry circuit is not sustained since the re-entrant excitation collides with the ablation lesion. The fibrillatory waves dissipate. (c) The model has returned to sinus rhythm. The ablation lesion disrupts the sinus wavefront, but does not induce fibrillation. Scale:  $100 \times 110$  nodes.

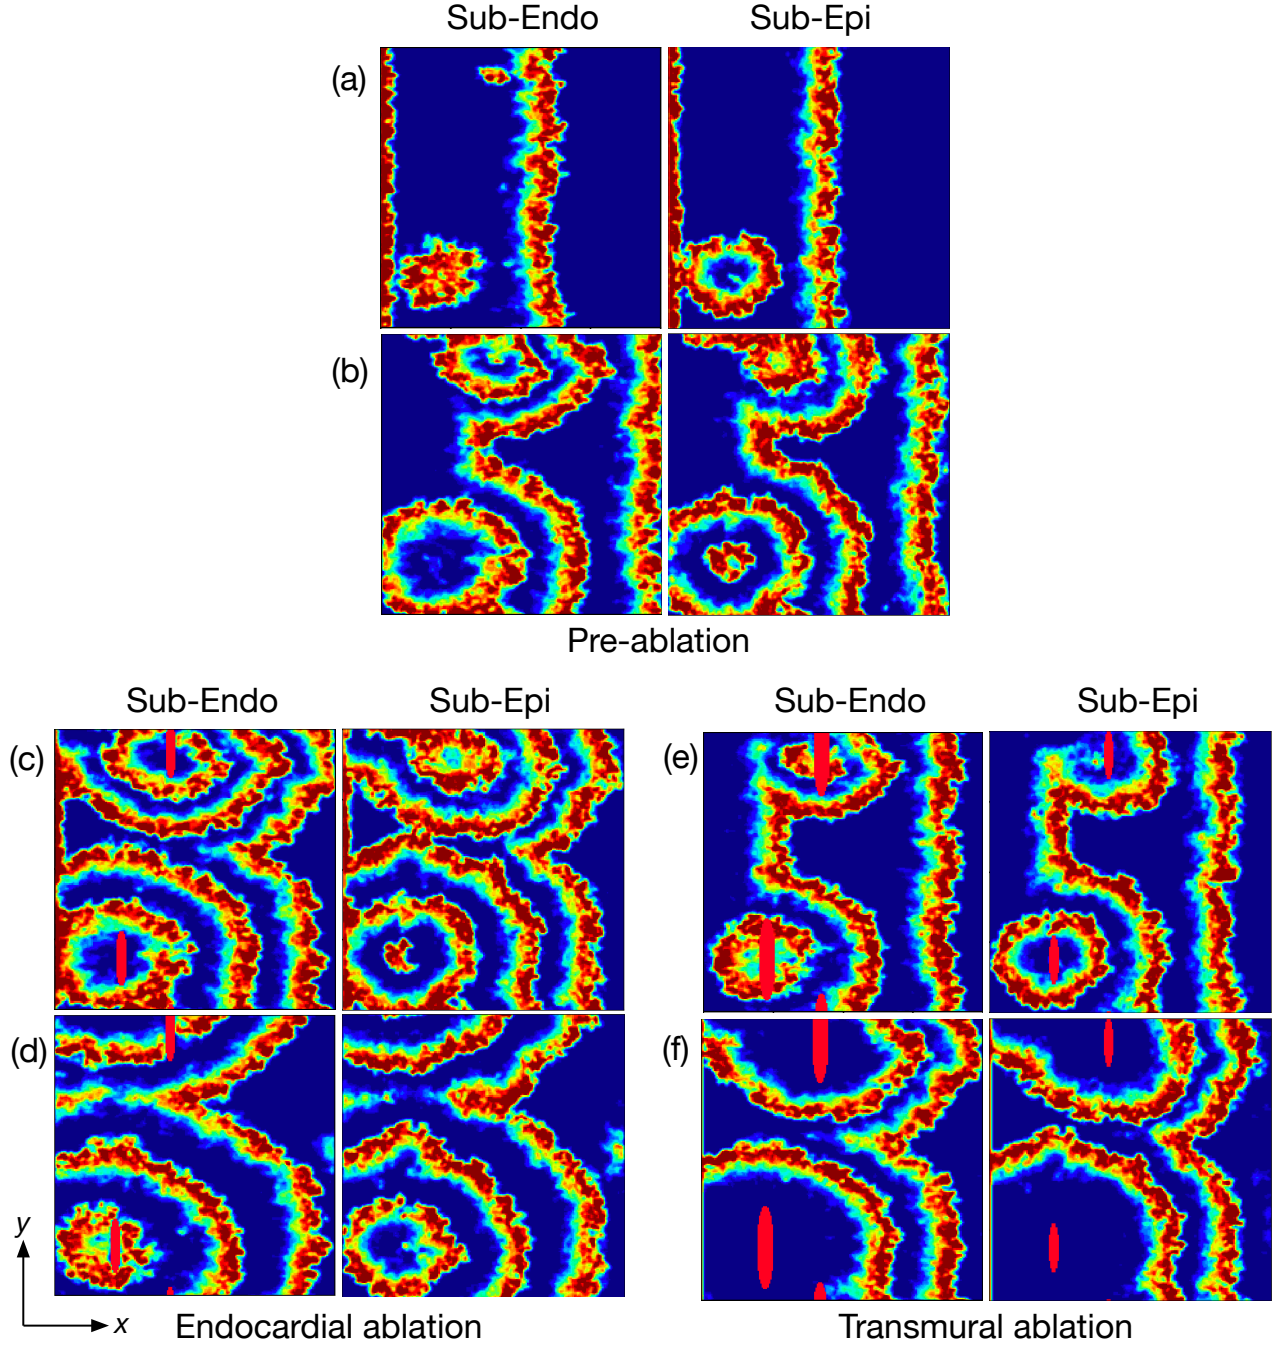

FIG. 14. A demonstration of ablation in a tissue with multiple drivers demonstrating how the ability to terminate fibrillatory activity is closely related to driver depth. (a) AF emerges in the bottom left corner from a re-entrant circuit near the epicardium, and (b) at the top of the tissue from a separate re-entrant circuit near the endocardium. (c) Two shallow ablations (solid red in bottom left and top centre) are applied to the endocardial surface at the locations of the re-entrant circuits penetrating part of the way into the tissue. (d) The circuit near the epicardium has not been destroyed by the ablation since the ablation has not penetrated far enough into the tissue. The circuit near the endocardium has been destroyed successfully. However, since an active circuit remains in the tissue, AF has not been terminated. (e) & (f) show the same ablation process as demonstrated in (c) & (d), however the ablation is now transmural, penetrating the full distance through the tissue. This is indicated by the solid red regions on the sub-epi view in (e) & (f). The ablations have successfully destroyed both re-entrant circuits. Hence, fibrillatory waves dissipate as shown in (f) and sinus rhythm will be restored. Note, transmural ablation is not always possible in clinical practice. Ablation lesions typically struggle to penetrate more than 2mm [8] into the atrial wall which can be up to 7mm thick in places [3]. Scale:  $200 \times 200$  nodes (full tissue).

- 
- [1] Lang, R. M. *et al.* Recommendations for chamber quantification: a report from the American Society of Echocardiography's Guidelines and Standards Committee and the Chamber Quantification Writing Group, developed in conjunction with the European Association of Echocardiography. *J. Am. Soc. Echocardiogr.* **18**, 1440–63 (2005).
  - [2] Maceira, A., Cosin-Sales, J., Roughton, M., Prasad, S. & Pennell, D. Reference left atrial dimensions and volumes by steady state free precession cardiovascular magnetic resonance. *J. Cardiovasc. Magn. Reson.* **12**, 65 (2010).
  - [3] Hansen, B. J. *et al.* Atrial fibrillation driven by micro-anatomic intramural re-entry revealed by simultaneous sub-epicardial and sub-endocardial optical mapping in explanted human hearts. *Eur. Heart J.* **36**, 2390–2401 (2015).
  - [4] Nakamura, K. *et al.* Left atrial wall thickness in paroxysmal atrial fibrillation by multislice-ct is initial marker of structural remodeling and predictor of transition from paroxysmal to chronic form. *Int. J. Cardiol.* **148**, 139 – 147 (2011).
  - [5] Luke, R. A. & Saffitz, J. E. Remodeling of ventricular conduction pathways in healed canine infarct border zones. *J. Clin. Investig.* **87**, 1594–602 (1991).
  - [6] Verheule, S. *et al.* Alterations in atrial electrophysiology and tissue structure in a canine model of chronic atrial dilatation due to mitral regurgitation. *Circulation* **107**, 2615–22 (2003).
  - [7] Christensen, K., Manani, K. A. & Peters, N. S. Simple model for identifying critical regions in atrial fibrillation. *Phys. Rev. Lett.* **114**, 028104 (2015).
  - [8] Kumar, S. *et al.* Better lesion creation and assessment during catheter ablation. *J. Atr. Fibrillation* **8**, 1189 (2015).
